# Supplementary material for: Visually Interpretable Subtask Reasoning for Visual Question Answering
Source: arXiv:2505.08084 source file (2025-05-12)
Supplement: Supplementary file 1 [file X_suppl.tex]

\clearpage
\setcounter{page}{1}
\maketitlesupplementary

\section{Rationale}
\label{sec:rationale}
